# Supplementary material for: Closing the gap towards end-to-end autonomous vehicle system
Source: arXiv:1901.00114 source file (2019-01-04)
Supplement: Supplementary file 1 [file appendix.tex]

\onecolumn
\newtheorem{theorem}{Theorem}[section]

\section{Supervised learning CVaR gradient}
\begin{theorem}{\textbf{CVaR gradient theorem.}}
Assume $\loss$ is a loss of a given network, parameterized by $\theta$, on a given dataset $\mathcal{D}$, and the CVaR is defined as in \eqref{def:cvar}. The gradient of the CVaR is given by: 
$$
\E{\ddtheta \loss\Bigg\lvert \loss\ge\nualpha}
$$
\end{theorem}
\begin{proof}
We are interested in a term for the gradient of the CVAR. We use the CVAR definition and follow the steps of \cite{trindade2007financial}, with slight adaptation to supervised learning framework. The proof is brought here as a whole to be self-contained.
\begin{align}
CVAR_\alpha(\loss)&=\nualpha+\frac{1}{1-\alpha}\cdot\E{(\loss-\nualpha)^+} \nonumber \\
&=\nualpha+\frac{1}{1-\alpha}\cdot\E{(\loss-\nualpha)\cdot1_{\loss\ge \nualpha}} \nonumber \\
&=\nualpha+\frac{1}{1-\alpha}\cdot\E{(\loss-\nualpha)\cdot1_{\loss-\nualpha\ge0}} \label{eqstar}
\end{align}	
Define $f(x)$ as:
$$
f(x) \triangleq x\cdot1_{x\ge0}
$$
and denoting $X=\loss-\nualpha$, we can write \eqref{eqstar} as:
\begin{align}
CVAR_\alpha(\loss)&=\nualpha+\frac{1}{1-\alpha}\cdot\E{f(X)} \label{cvarbeforegradient}
\end{align}
Note that $f'(X)=1_{x\ge 0}$, and that $f(X)$ is Lipschitz continuous.
\newline
We now compute the gradient w.r.t $\theta$ on \eqref{cvarbeforegradient}:
\begin{align*}
\ddtheta CVAR_\alpha(\loss)&=\ddtheta\nualpha+\frac{1}{1-\alpha}\cdot\ddtheta\E{f(x)}
\end{align*}
Using transitivity of derivation and expectation:
\begin{align*}
\ddtheta CVAR_\alpha(\loss)&=\ddtheta\nualpha+\frac{1}{1-\alpha}\cdot\ddtheta\E{f(X)}\\
&\underset{transitivity}{=}\ddtheta\nualpha+\frac{1}{1-\alpha}\cdot\E{f'(X)\cdot\ddtheta {X}}\\
&=\ddtheta\nualpha+\frac{1}{1-\alpha}\cdot\E{1_{X\ge0}\cdot\ddtheta{X}}\\
&\underset{\text{switch vars}}{=}
\ddtheta\nualpha+\frac{1}{1-\alpha}\cdot\E{1_{\loss-\nualpha\ge0}\cdot\ddtheta{\brackets{\loss-\nualpha}}}\\
&=\ddtheta\nualpha+\frac{1}{1-\alpha}\cdot\E{1_{\loss\ge\nualpha}\cdot\brackets{\ddtheta \loss-\ddtheta\nualpha}}\\
&\underset{(**)}{=}
\E{\ddtheta \loss\Bigg\lvert \loss\ge\nualpha}
\end{align*} 
The last line results in the following formula for CVAR gradient:
\[
\boxed{\ddtheta CVAR_\alpha(\loss)=\E{\ddtheta \loss\Bigg\lvert \loss\ge\nualpha}}
\]
One can simply estimate this gradient using samples from $D$.

We now prove (**). For simplicity, we define:
$G(\loss)\triangleq\ddtheta \loss $, $a=\ddtheta\nualpha$. Note that $a$ is independent of $\loss$.
Thus we can write:
\begin{align*}
\ddtheta\nualpha+\frac{1}{1-\alpha}\cdot\E{1_{\loss\ge\nualpha}\cdot\brackets{\ddtheta \loss-\ddtheta\nualpha}}&\triangleq a+\frac{1}{1-\alpha}\E{1_{\loss>\nualpha\cdot(G(\loss)-a)}}\\
\end{align*}
thus,
\begin{align}
a+\frac{1}{1-\alpha}\E{1_{\loss>\nualpha\cdot(G(\loss)-a)}}
&=a+\frac{1}{1-\alpha}\int_{-\inf}^{\inf} 1_{\loss>\nualpha}\cdot(G(\loss)-a)f_Z(z)dz\nonumber\\
&=a+\frac{1}{1-\alpha}\int_{\nualpha}^{\inf}(G(\loss)-a)f_Z(z)dz
\label{condprob}
 \end{align}
Note that 
$$
f_{\loss>\nualpha}=\begin{cases} 
1 & \text{w.p  } 1-\alpha\\
0 & \text{w.p  } \alpha
\end{cases}
$$
and 
$$
f_{\loss,\loss>\nualpha}=\begin{cases} 
f_Z(z) & \text{if } z\ge\nualpha \\
0 & \text{if } z\le\nualpha
\end{cases}
$$
thus we can write \eqref{condprob} as:
\begin{align*}
\eqref{condprob}&=a+\int_{\nualpha}^{\inf}(G(\loss)-a)\frac{f_Z(z)}{1-\alpha}dz\\
&=a+\int_{-\inf}^{\nualpha}(G(\loss)-a)\frac{ 0}{\alpha}dz+\int_{\nualpha}^{\inf}(G(\loss)-a)\frac{f_Z(z)}{1-\alpha}dz\\
&=a+\int_{-\inf}^{\inf} (G(\loss)-a) \frac{f_{\loss,\loss>\nualpha}}{f_{\loss>\nualpha}}dz\\
&=a+\int_{-\inf}^{\inf} (G(\loss)-a) f_{\loss|\loss>\nualpha}dz\\
&=\int_{-\inf}^{\inf} G(\loss) f_{\loss|\loss>\nualpha}dz\\
&=\E{G(\loss)|\loss>\nualpha}\\
&=\E{\ddtheta\Bigg\lvert \loss>\nualpha}\\
\end{align*}

\end{proof}
