# Supplementary material for: Closing the gap towards end-to-end autonomous vehicle system
Source: arXiv:1901.00114 source file (2019-01-04)
Supplement: Supplementary file 6 [file supplemetary_material.tex]

\section{Supplementary material}
	We demonstrate closed-loop driving performance of our end-to-end system in TORCS simulator.
	\\We present performance in a highway scenario with static opponents (discussed throughout the paper). 
	\\We also provide first results in a dynamic scenario (highway with dynamic opponents).
	Video is available at \changeurlcolor{blue}\href{http://www.youtube.com/watch?v=7ecFccoOyxc}{http://www.youtube.com/watch?v=7ecFccoOyxc}
